# Supplementary material for: Wheeler: A Three-Wheeled Input Device for Usable, Efficient, and Versatile Non-Visual Interaction
Source: arXiv:2408.13166 source file (2024-08-23)
Supplement: Supplementary file 1 [file appendix-h-nav-theory.tex]

\section{Theoretical Gain in Navigating UI Hierarchy with \texttt{H-nav} Mode Compared to Screen Readers}
\label{subsec:hnav_theory}
\fx{still needs work}

Blind users use a combination of keyboard and screen readers (SR) to navigate different application menus, which often have multi-level hierarchies.
\sysname{}'s \hnav{} mode is designed specifically to improve such users' performance in the aforementioned task.
In this section, through theoretical analysis, we show that the time complexity of multi-level menu navigation using \sysname{}'s \hnav{} mode can be significantly better than that of using the (keyboard+SR) combo.

\begin{figure*}[!ht]
    \centering
    \begin{minipage}[t]{.49\textwidth}
    \centering
    \includegraphics[width=\columnwidth,center]{figures/baseline-tree.pdf}
    \small{(a)}
    \end{minipage}
    \hspace{2pt}
    \begin{minipage}[t]{.49\textwidth}
    \centering
    \includegraphics[width=\columnwidth,center]{figures/baseline-path.pdf}
    \small{(b)}
    \end{minipage}
    \caption{(a) A sample hierarchy tree in a (keyboard + Screen Reader)-based interaction. The tree consists of three types of edges: forward, backward, and cross edges.
    Each edge has an associated cost that is shown alongside the edge.
    We consider that 7 is the currently selected node, and the user's target destination is node 17.
    (b) shows the edges (highlighted in green) required to create the shortest path from 7 to 17, with a total cost of $3\alpha + \beta + 2\gamma$.}
    \label{fig:theoretical_complexity_baseline}
\end{figure*}

\begin{figure*}[!ht]
    \centering
    \begin{minipage}[t]{.49\textwidth}
    \centering
    \includegraphics[width=\columnwidth,center]{figures/wheeler-tree.pdf}
    \small{(a)}
    \end{minipage}
    \hspace{2pt}
    \begin{minipage}[t]{.49\textwidth}
    \centering
    \includegraphics[width=\columnwidth,center]{figures/wheeler-path.pdf}
    \small{(b)}
    \end{minipage}
    \caption{(a) A sample hierarchy tree when using \sysname{}. The tree consists of two types of edges: cross and teleport edges.
    Cross edges cost $\gamma$, and teleport edges have 0 cost.
    7 and 17 are the current and target nodes, just like in Figure~\ref{fig:theoretical_complexity_baseline}.
    (b) shows the edges (highlighted in green) required to create the shortest path from 7 to 17, with a total cost of $2\gamma$.}
    \label{fig:theoretical_complexity_wheeler}
\end{figure*}

\subsection{Assumptions}
To facilitate our analysis, we assume the following interaction flow:

\begin{enumerate}
    \item We assume that a blind screen reader user is tasked with finding a menu item in an accessible application (e.g., Microsoft Word) that the user has not used before. As the traversal of an application menu or computer storage happens sequentially in a hierarchical structure, we can demonstrate the user's interaction with the menu items using an \textbf{m-ary} tree.
    Every node in the tree would represent a UI item in the application menu.
    On the other hand, every edge in the tree would represent a valid movement path between two nodes.
    
    \item Even if the first item on the first-level menu is the target item, we assume that the user would need at least one action (i.e., wheel rotation) to reach the target. As such, at the very beginning, the user's cursor remains at a virtual {\textbf{ROOT}} node as shown in Figure~\ref{fig:theoretical_complexity_baseline}. 
    Moreover, we assume the tree has a depth of 3 for simplicity.

    \item The user traverses the menu and sub-menu items one at a time and listens to the screen reader’s text-to-speech information to verify their current position.
    Consequently, each interaction takes a certain amount of time to be completed. 
    We call the required interaction time ``cost''.
    
    \item As the user gains experience by traversing a certain application's menu, we assume that their performance (i.e., task completion time) will improve over time. 
    
    \item We assume that looking for an item in an application menu is similar to searching for a node in an \textbf{m-ary} tree.
    The only exceptions to this notion are leaf nodes under the same parent; in other words, nodes that are siblings.
    In a tree traversal, going from one sibling node to another requires returning to the parent first, as there is no direct path between the siblings. However, in traversing a UI, a user can move directly between all the nodes under a certain parent menu item.
    As such, the tree structure in our consideration would allow movement between siblings.

\end{enumerate}

\subsection{Interaction Types and Associated Costs}
To move from one node to another, the user has to perform certain actions (e.g., pressing a key, rotating \sysname{}'s wheels).
These actions are represented using edges in our tree.
We assume the following types of edges and explain their associated costs:
        
\begin{itemize}

    \item \textit{Forward Edge.} 
    These edges are used when navigating to the next level in a menu hierarchy. As such, they are unidirectional and point towards a child from a parent.
    These edges are only needed when the user is using a screen reader. They are not needed when \sysname{} is used, as the user can use the cursor for the next level instead of moving the current cursor from the current level to one level down.
    The task underneath a forward edge involves choosing the next option using the keyboard, listening to the screen reader’s output, and understanding whether the user is at the target. We assume that the forward edge has a cost of $\alpha$. 
    
    \item \textit{Backward Edge.}
    These are also unidirectional edges and point towards a parent from a child.
    They are used when navigating to the previous level in a menu hierarchy or terminating the search by returning to the \textbf{ROOT} using the \textbf{ESC} key.  Like before, these edges are only needed when the user uses a screen reader.
    We assume that the backward edge has a cost of $\beta$.

    \item \textit{Cross Edge.} Cross edges are lateral and allow movement between siblings in a tree.
    These edges are used when the user uses a screen reader and \sysname{}.
    We assume the cost of cross edges to be $\gamma$.

    \item \textit{Teleport Edge.} These edges automatically transfer the (n+1)-th wheel to the node's first child selected by the n-th wheel.
    Recall that \sysname{} allows three distinct cursors, one for each wheel. 
    As such, for the tree in Figure \ref{fig:theoretical_complexity_wheeler}, \wa{} would be assigned to level 1, \wb{} would be assigned to level 2, and \wc{} would be assigned to level 3.
    Therefore, using \wa{}, the user can access nodes 8 and 16 in level 1.
    Similarly, if \wa{} is at 8, the user can access 6 and 10 using \wb{}, 
    and if \wb{} is at 10, the user can access 9 and 11 using \wc{}.
    Now, if the user moves \wa{} from 8 to 16, \wb{}'s cursor would automatically move to 14, the first child of 16, and \wc{}'s cursor would automatically move to 13, the first child of 14.
    As these cursor transfers are instantaneous and do not require any extra user effort, we call them teleport edges and assume they have zero cost. 
    
\end{itemize}

\subsection{Performance Comparison of \hnav{} Mode and Screen Readers}

Let us take a closer look at Figures~\ref{fig:theoretical_complexity_baseline}a and ~\ref{fig:theoretical_complexity_wheeler}a.
Both figures work with the same hierarchy tree but present the views of two different systems.
Figure~\ref{fig:theoretical_complexity_baseline}a shows the hierarchy tree view of a screen reader-based navigation system, while Figure~\ref{fig:theoretical_complexity_wheeler}a shows the hierarchy tree view when the user uses \sysname{}. 
The goal in both systems is to get to node 17 (i.e., destination) from node 7 (i.e., source).

Figure~\ref{fig:theoretical_complexity_baseline}b shows the shortest path from node 7 to 17 (highlighted in green).
Considering the associated costs for each edge along the path, the total cost becomes $\alpha + \beta + \gamma + \alpha + \gamma + \alpha$, i.e., $3\alpha + \beta + 2\gamma$.

Figure~\ref{fig:theoretical_complexity_wheeler}b shows the shortest path from node 7 to 17 (highlighted in green).
Thanks to multiple cursors in \sysname{}, the forward and backward edges are unnecessary in this scenario.
When the user is at node 7, which is at level 3 and assigned to \wc{}, \wb{} must be at node 6, and \wa{} must be at node 8.
Thus, moving \wa{} just once, the user gets to the target node's grandparent 16.
When \wa{} is at 16, \wb{} automatically moves to its first child, 14. Then, the user has to rotate \wb{} once to get to 18.
When the user moves to 18, \wc{} automatically moves to 17, the target destination.
In this scenario, the user needs only two wheel movements.
In terms of cost, it sums up to $\gamma + 0 + \gamma$, i.e., $2\gamma$, which is substantially smaller than the cost we got with screen reader-based navigation.
