# Supplementary material for: Wheeler: A Three-Wheeled Input Device for Usable, Efficient, and Versatile Non-Visual Interaction
Source: arXiv:2408.13166 source file (2024-08-23)
Supplement: Supplementary file 2 [file appendix.tex]

\section{Appendix: Mathematical Derivation}

% \section{Mathematical Derivation}
% 

\subsection{Equation~\ref{eq:first}}
\begin{equation}
    \begin{aligned}
    ID_{fitts} - ID_{\fnav{}} & \approx 0 \\
     \log_{2} {\frac{2d}{W}} - \log_{2} {\frac{2(|d_1| + |d_2|)}{W}} & \approx 0 \\
     \log_{2} \frac{{\frac{2d}{W}}}{{\frac{2(|d_1| + |d_2|)}{W}} }  & \approx 0 \\
     \log_{2} \frac{d}{|d_1| + |d_2|}  & \approx 0\\
     \frac{d}{|d_1| + |d_2|}  & \approx 1 \\
     (|d_1| + |d_2|) & \approx d
    \end{aligned}
    \label{eq:first}
\end{equation}

\subsection{Equation~\ref{eq:second}}
Now, we need to compress $d_1$ and $d_2$ by increasing the cursor movement speed, $s$.
\begin{equation}
    \begin{aligned}
    \frac{|d_1|}{s} + \frac{|d_2|}{s} & = d \\
    \frac{d*\cos(\theta)}{s} + \frac{d*\sin(\theta)}{s} & = d \\
    \frac{\cos(\theta)}{s} + \frac{\sin(\theta)}{s} & = 1 \\
    \frac{\cos(\theta) + \sin(\theta)}{s} & = 1 \\
    \end{aligned}
    \label{eq:second}
\end{equation}
